# Supplementary material for: Parallelism and Time in Hierarchical Self-Assembly
Source: arXiv:1104.5226 source file (2017-02-12)
Supplement: Supplementary file 1 [file appendix.tex]

\section{Technical Appendix}
\label{sec-appendix}

\subsection{Formal Definition of Abstract Tile Assembly Model}
\label{sec-tam-formal}
\input{tam-formal}

\subsection{Construction of Highly Parallel Square}
\label{sec-app-parallel-square}

\paragraph{Comparison of Parallelism in the Hierarchical aTAM with Staged Self-Assembly.}
\CompareToStaged

\paragraph{Definition of Parallelism in the Hierarchical aTAM.}
\ParallelDefn

\paragraph{Full Construction of Highly Parallel Square.}
\FigNonPowTwo
\FigBlock
\begin{proof}[Proof of Theorem~\ref{thm-hierarchical-square}.]
\ProofParallelSquare
\end{proof}

\subsection{Time Complexity of Self-Assembly}
\label{sec-app-time-complexity-general}

\unrealisticHierarchical

\subsubsection{Explanation of Propensity Definitions}\label{sec-propensity-explanation}
\propensityExplanation

\subsubsection{Time Lower Bound for Seeded Systems}
\label{app-sec-seeded-lower-bound}
The following is a more formal statement of Theorem~\ref{thm-seeded-time-lower-bound}.

\seededLowerBoundFormal

\paragraph{Theorem~\ref{thm-seeded-time-lower-bound} (Formal Statement).}
  {\it \seededLowerBoundFormalStatement}

\begin{proof}[Proof of Theorem~\ref{thm-seeded-time-lower-bound}.]
  \ProofSeededTimeLowerBound
\end{proof}

\subsubsection{Time Complexity of Hierarchical Systems}
\label{sec-app-hier-partial-order-slow}

\modelJustification

\LemmaConserveMass

\begin{proof}[Proof of Theorem~\ref{thm-hier-partial-order-slow}.]
  \ProofHierPartialOrderSlow
\end{proof}

\subsection{Assembly of a Shape in Time Sublinear in its Diameter}
\label{app-sec-fast-rectangle}
\fastSquareSection

\subsection{Open Questions}
\label{sec-conclusion}
\openQuestions
